# Supplementary material for: Quantized Zero Dynamics Attacks against Sampled-data Control Systems
Source: arXiv:2303.11982 source file (2023-03-21)
Supplement: Supplementary file 1 [file appendix.tex]

\begin{proof}
We denote an arbitrary unstable eigenvalue of $S$ as $\lambda$ and corresponding eigenvector as $p~(\|p\|_2=1)$. Let initial value $\eta^a[0]=\kappa p$ in \eqref{eq:no:zda} where $\kappa$ is real number. We denote $\Delta\eta[k]:=\eta_{u+a}[k]-\eta_u[k]$ and  $\Delta\zeta[k]:=\zeta_{u+a}[k]-\zeta_u[k]$, then outputs error coincides with the output of following system.
\begin{equation}
    \begin{split}
        \Delta\eta[k+1]&=S\Delta\eta[k]+P\Delta\zeta[k],\\
        \Delta\zeta[k+1]&=\phi\Delta\zeta[k]+\psi\Delta\eta[k]+ga[k],\\
        y_{u+a}[k]-y_u[k]&=\Delta\zeta[k].
    \end{split}\label{eq:no:normdiff}
\end{equation}
In accordance with \eqref{eq:no:zda} and \eqref{eq:no:normdiff}, outputs error is calculated by next equation where $\Delta\tilde{\eta}[k]:=\Delta\eta[k]-\eta^a[k]$.
\begin{equation}
    \begin{split}
        \Delta\tilde{\eta}[k+1]&=S\Delta\tilde{\eta}[k]+P\Delta\zeta[k],\\
        \Delta\zeta[k+1]&=\phi\Delta\zeta[k]+\psi\Delta\tilde{\eta}[k],\\
        y_{u+a}[k]-y_u[k]&=\Delta\zeta[k].
    \end{split}\label{eq:no:normdiff2}
\end{equation}
If we denote the transform matrix into normal form as $M$, then
\begin{equation}
    \begin{bmatrix}
        \eta[k]\\
        \zeta[k]
    \end{bmatrix}=Mx[k].\label{eq:no:statetrans}
\end{equation} 
At this time, the response of \eqref{eq:no:normdiff2} is equivalent to the initial condition response of \eqref{eq:no:dsys} where initial state is $x[0]=M^{-1}[(\eta^a)^T[0],0]^T$. Therefore,
\begin{equation}
    \begin{split}
    y_{u+a}[k]-y_u[k]&=CA^kM^{-1}\begin{bmatrix}
    -\eta^a[0] \\
    0
    \end{bmatrix}\\
    &=\kappa CA^kM^{-1}\begin{bmatrix}
    -p \\
    0
    \end{bmatrix}.
    \end{split}\label{eq:no:diffy}
\end{equation}
Since $A$ is a stable matrix, $\sup_{k}\left|CA^kM^{-1}[p^T,0]^T\right|$ is finite value. Hence, if we let
\begin{equation}
    \kappa\leq\frac{\epsilon}{\sup\limits_{k}\left|CA^kM^{-1}\begin{bmatrix}
p \\
0
\end{bmatrix}\right|},
\end{equation}
the attack signals $\{a[k]\}_{k=0}^{\infty}$ is $\epsilon$-stealthy.\\
Let us move into states difference $x_{u+a}[k]-x_u[k]$. In accordance with \eqref{eq:no:statetrans} and definition of $\Delta\tilde{\eta}[k]$,
\begin{equation*}
    \begin{split}
        x_{u+a}[k]-x_u[k]&=M^{-1}\begin{bmatrix}
        \Delta\eta[k] \\
        \Delta\zeta[k]
        \end{bmatrix}\\
        &=M^{-1}\begin{bmatrix}
        \eta^a[k] \\
        0
        \end{bmatrix}+M^{-1}\begin{bmatrix}
        \Delta\tilde{\eta}[k] \\
        \Delta\zeta[k]
        \end{bmatrix}.
    \end{split}
\end{equation*}
Considering triangle inequality, we obtain following inequality.
\begin{equation}
    \begin{split}
        \left\|x_{u+a}[k]-x_u[k]\right\|_2\geq\left\|M^{-1}\begin{bmatrix}
        \eta^a[k] \\
        0
        \end{bmatrix}\right\|_2-\left\|M^{-1}\begin{bmatrix}
        \Delta\tilde{\eta}[k] \\
        \Delta\zeta[k]
        \end{bmatrix}\right\|_2
    \end{split}\label{eq:no:diffs1}
\end{equation}
From \eqref{eq:no:normdiff2}, $[\Delta\tilde{\eta}^T[k],\Delta\zeta[k]]^T=MA^kM^{-1}[(\eta^a)^T[0],0]^T$.\\Therefore, the second term of \eqref{eq:no:diffs1} satisfies
\begin{equation*}
    \left\|A^kM^{-1}\begin{bmatrix}
        \eta^a[0] \\
        0
        \end{bmatrix}\right\|_2\leq\sup\limits_k\left\|A^kM^{-1}\begin{bmatrix}
        p \\
        0
        \end{bmatrix}\right\|_2\kappa<\infty.
\end{equation*}
Next, we claim the first term of \eqref{eq:no:diffs1} diverges. Because $\eta^a[k]=S^k\eta[0]=\lambda^k\kappa p$,  
\begin{equation*}
    \left\|M^{-1}\begin{bmatrix}
        \eta^a[k] \\
        0
        \end{bmatrix}\right\|_2=\left\|M^{-1}\begin{bmatrix}
        p \\
        0
        \end{bmatrix}\right\|_2\lambda^k\kappa\rightarrow\infty~(k\rightarrow\infty).
\end{equation*}
It means the right hand side of \eqref{eq:no:diffs1} diverges as $k\rightarrow\infty$. Consequently, $\left\|x_{u+a}[k]-x_u[k]\right\|_2$ also diverges.
\end{proof}

\begin{theo}
It is assumed that $\{H_k\}_{k=0}^{\infty}$ and quantization width $d$ are given. If the quantized attack $\{b[k]\}_{k=0}^{\infty}$ generated by \eqref{eq:no:dzdag} for an $\epsilon\geq|CB|d$, then this attack is $\left(\epsilon+|CB|\Delta\right)$-stealthy. Moreover, this attack is $\{H_k\}_{k=0}^{\infty}$-disruptive if the following conditions are satisfied:
\begin{itemize}
    \item Consider the Jordan decomposition of $\left(A-\frac{BCA}{CB}\right)=P\Lambda P^{-1}$. Moreover, let the diagonal elements of $\Lambda$ be $\sigma_1,\ldots,\sigma_n$ and $\sigma_l,\ldots,\sigma_n$ be unstable ones. Then at least one of the $l-th$ through the last element of $B':=P^{-1}B$ is not $0$.
\end{itemize}
\end{theo}
\begin{proof}
States difference and outputs difference are $x_{v+b}[k]-x_v[k]=z[k]$, $y_{v+b}[k]-y_v[k]=Cz[k]$ respectively. Introducing  $w[k]:=(-\frac{CA}{CB}z[k]+\frac{\sign(CB)\epsilon}{CB}+\Delta)-b[k]$, \eqref{eq:no:dzdag} becomes
\begin{equation}
    z[k+1]=\left(A-\frac{BCA}{CB}\right)z[k]+B\left(\frac{\sign(CB)\epsilon}{CB}+\Delta-w[k]\right)
\end{equation}
where $0<w[k]\leq d$. Thus, 
\begin{equation}
    z[k]=\sum_{l=0}^{k-1}\left(A-\frac{BCA}{CB}\right)^{k-l-1}B\left(\frac{\sign(CB)\epsilon}{CB}\Delta-w[l]\right).\label{eq:no:zk}
\end{equation}
Because $C\left(A-\frac{BCA}{CB}\right)=0$, $Cz[k]=\sign(CB)\epsilon+CB\Delta-CBw[k-1]$ for all $k\geq1$. If $\epsilon\geq|CB|d$, $-\left(\epsilon+|CB|\Delta\right)\leq|Cz[k]|\leq\epsilon+|CB|\Delta$. It means the attack $\{b[k]\}_{k=0}^{\infty}$ is $\left(\epsilon+|CB|\Delta\right)$-stealthy.\par
Next, we look at the square norm of $z[k]$. Since $\epsilon\geq|CB|d$, $w'[k]:=\frac{\sign(CB)}{CB}\epsilon+\Delta-w[k]\geq\Delta$. Then, the equation \eqref{eq:no:zk} is:
\begin{equation}
    z[k]=\sum_{l=0}^{k-1}P\Lambda^{k-l-1}B'w'[l].\label{eq:no:zk2}
\end{equation}
By the assumption, there exist the last nonzero element of $B'$, whose index is equal or greater than $l$. Here, we denote this index $l^*$. Then $P^{-1}z[k]$ is:
\begin{equation}
    P^{-1}z[k]=\begin{bmatrix}
    *\\
    \vdots\\
    *\\
    \sum_{l=0}^{k-1}\sigma_{l^*}^{k-l-1}B_{l^*}'w[l]\\
    0\\
    \vdots\\
    0
    \end{bmatrix}.\label{eq:no:zk2}
\end{equation}
The square norm of $z[k]$ is satisfies the following inequalities:
\begin{equation*}
    \begin{split}
        \left\|z[k]\right\|_2&\geq\left\|P\right\|_2\left\|P^{-1}z[k]\right\|_2\\
        &\geq\left\|P\right\|_2\left|\sum_{l=0}^{k-1}\sigma_{l^*}^{k-l-1}B_{l^*}'w'[l]\right|\rightarrow\infty.
    \end{split}
\end{equation*}
Hence, $\left\|x_{v+b}[k]-x_v[k]\right\|_2$ also diverges. Consequently, the attack $\{b[k]\}_{k=0}^{\infty}$ is  $\{H_k\}_{k=0}^{\infty}$-disruptive.
\end{proof}
